# Supplementary material for: Uncertain Transport in Unsteady Flows
Source: arXiv:2009.04531 ancillary file (2020-08-30)
Supplement: Supplementary file 1 [file supplementary_document.pdf]

# Uncertain Transport in Unsteady Flows
# Supplementary Material

Tobias Rapp* Carsten Dachsbacher†

Institute for Visualization and Data Analysis
Karlsruhe Institute of Technology

## 1 Introduction

We present additional results that are not in the main paper. The definition and further results for the double gyre flow are given in Sect. 2. In Sect. 3, we perform more evaluations on the Red Sea dataset. We present the heated cylinder dataset in Sect. 4, where we study uncertainty due to data reduction. Lastly, we compare the FTLE and DBS of the deterministic flow around corners in Sect. 5.

## 2 Double Gyre

The analytic double gyre flow is defined as

$$v(x,y,t) = \begin{pmatrix} -\pi A \sin(f(x,t)\pi)\cos(\pi y) \\ \pi A \cos(f(x,t)\pi)\sin(\pi y)\frac{\partial}{\partial x} f(x,t) \end{pmatrix}, \quad (1)$$

where

$$\begin{aligned} f(x,t) &= a(t)x^2 + b(t)x \\ a(t) &= \varepsilon \sin(\omega t) \\ b(t) &= 1 - 2\varepsilon \sin(\omega t). \end{aligned} \quad (2)$$

We set $A = 0.1$, $\omega = 2\pi/10$, and $\varepsilon = 0.1$.

The forward FTLE of this flow is shown in Fig. 1 (a) and the forward DBS is shown in (b). Now, we add different amounts of isotropic Gaussian noise. The transport uncertainty is thus constant everywhere and the DBS is not affected by changing the absolute scale of noise. However, for increasing amounts of noise the assumption of small deviations is no longer valid. The behavior of the uncertain flow is visualized by stochastic integration of a large amount of particles and mapping their density in (c), (g), and (k), which illustrates the separatrices in the flow. For small deviations, these visualizations align with the DBS. With increasing amounts of noise, barriers with a low DBS value are no longer visible. The FTLE-D, obtained by averaging the right Cauchy-Green strain tensor, and the probabilistic D-FTLE from Guo et al. [2] similarly illustrate the influence of adding more noise.

In the main paper, we employ the double gyre dataset reduced to a discrete grid of size $[256 \times 128 \times 10]$ and estimated a Gaussian error model. The resulting variance and covariance averaged over time are visualized in Fig. 2. The amount of variance (d, e) and covariance (f) varies periodically. In contrast, the transport uncertainty shown in the main paper directly visualizes the impact of the uncertainty on the advected tracer particles.

## 3 Red Sea

The forward DBS of the Red Sea dataset is shown in Fig. 3 (a), integrated over the same 182 hours as in the main paper. Additionally, we visualize the mean concentration of salinity in the upper layers of the ocean at the beginning (b) and the end of the time interval (c). The diffusion of salinity visibly aligns with the most significant transport barriers identified by the forward DBS. The transport uncertainty shown in (d) indicates a high uncertainty in the lower right part of the dataset, the gulf of Aden.

Fig. 4 illustrates the time averaged variance of the velocities, salinity, and temperature. For most quantities, the variance is highest in the gulf of Aden, corresponding to the transport uncertainty. The DBS depicts strong transport barriers and enhancers in this region that correspond to the diffusion of salinity and temperature.

The forward FTLE of the mean flow is shown in Fig. 5 (a). Although the FTLE contains more noise than the DBS in Fig. 3 (a), it indicates similar structures in the Red Sea. In the higher variance region in the Gulf of Aden, the differences are more pronounced. Since the FTLE only uses the mean flow, the results do not take the uncertainty into account. In comparison, the FTLE-D in Fig. 5 (b) is computed from the stochastic flow. The FTLE-D is not as noisy as the FTLE, but requires a significant amount of computational effort to achieve this. In the gulf of Adan, the FTLE-D shows a large amount of finer features. The visible structures in the temperature and salinity are barely, if at all, present.

## 4 Heated Cylinder

This dataset consists of a 2D time-dependent flow generated by a heated cylinder using the Boussinesq approximation. The dataset is due to Günther et al. [1] and was simulated using the Gerris flow solver [3]. It shows a turbulent plume that contains several small vortices rotating around each other. The dataset is stored in a regular grid of resolution $[150 \times 450 \times 2001]$.

The backward FTLE of the time interval $[10,0]$ is shown in Fig. 6 (a). We have reduced the temporal resolution of the data set to 100 time steps and estimated the mean and covariance matrix in each grid cell. We visualize attractors in the uncertain flow in (b) by integrating particles forward in time and visualizing their density. The DBS of the stochastic flow is shown in (c) and the transport uncertainty in (d). The FTLE-D is shown in (e). The probabilistic D-FTLE is not shown here, but corresponds closely to the FTLE-D.

The uncertain flows indicates a changed flow behavior compared to the FTLE in (a) since some vortices have been stretched or rotated. Since the DBS incorporates the relative scaling and anisotropy, these changes are taken into account without requiring stochastic numerical integration. Moreover, the DBS tends to smooth out the center of vortical regions, in correspondence to the density visualization shown in (b) and the transport uncertainty in (d), which is not the case for the FTLE-D.

## 5 Flow Around Corners

This flow around two cylinders and corners has been simulated using the Gerris flow solver [3] and is due to Baeza Rojo and Günter [4]. Here, we visualize the deterministic flow without explicitly constructing an error model, i.e. we set $D = I$ and assume $s \to 0$. Fig. 7 shows the backward FTLE (a) and the DBS (b) in the time interval $[10,5]$. The quantities are similar, but not identical. For example, the DBS smooths out fine-scale features inside vortical regions.

*e-mail: tobias.rapp@kit.edu
†e-mail: dachsbacher@kit.edu

# References


[1] T. Günther, M. Gross, and H. Theisel. Generic objective vortices for flow visualization. *ACM Transactions on Graphics (Proc. SIGGRAPH)*, 36(4):141:1–141:11, 2017.

[2] H. Guo, W. He, T. Peterka, H. Shen, S. M. Collis, and J. J. Helmus. Finite-time Lyapunov exponents and Lagrangian coherent structures in uncertain unsteady flows. *IEEE Transactions on Visualization and Computer Graphics*, 22(6):1672–1682, 2016. doi: 10.1109/TVCG.2016.2534560

[3] S. Popinet. Free computational fluid dynamics. *ClusterWorld*, 2(6), 2004.

[4] I. B. Rojo and T. Günther. Vector field topology of time-dependent flows in a steady reference frame. *IEEE Transactions on Visualization and Computer Graphics*, 26(1):280–290, 2020. doi: 10.1109/TVCG.2019.2934375

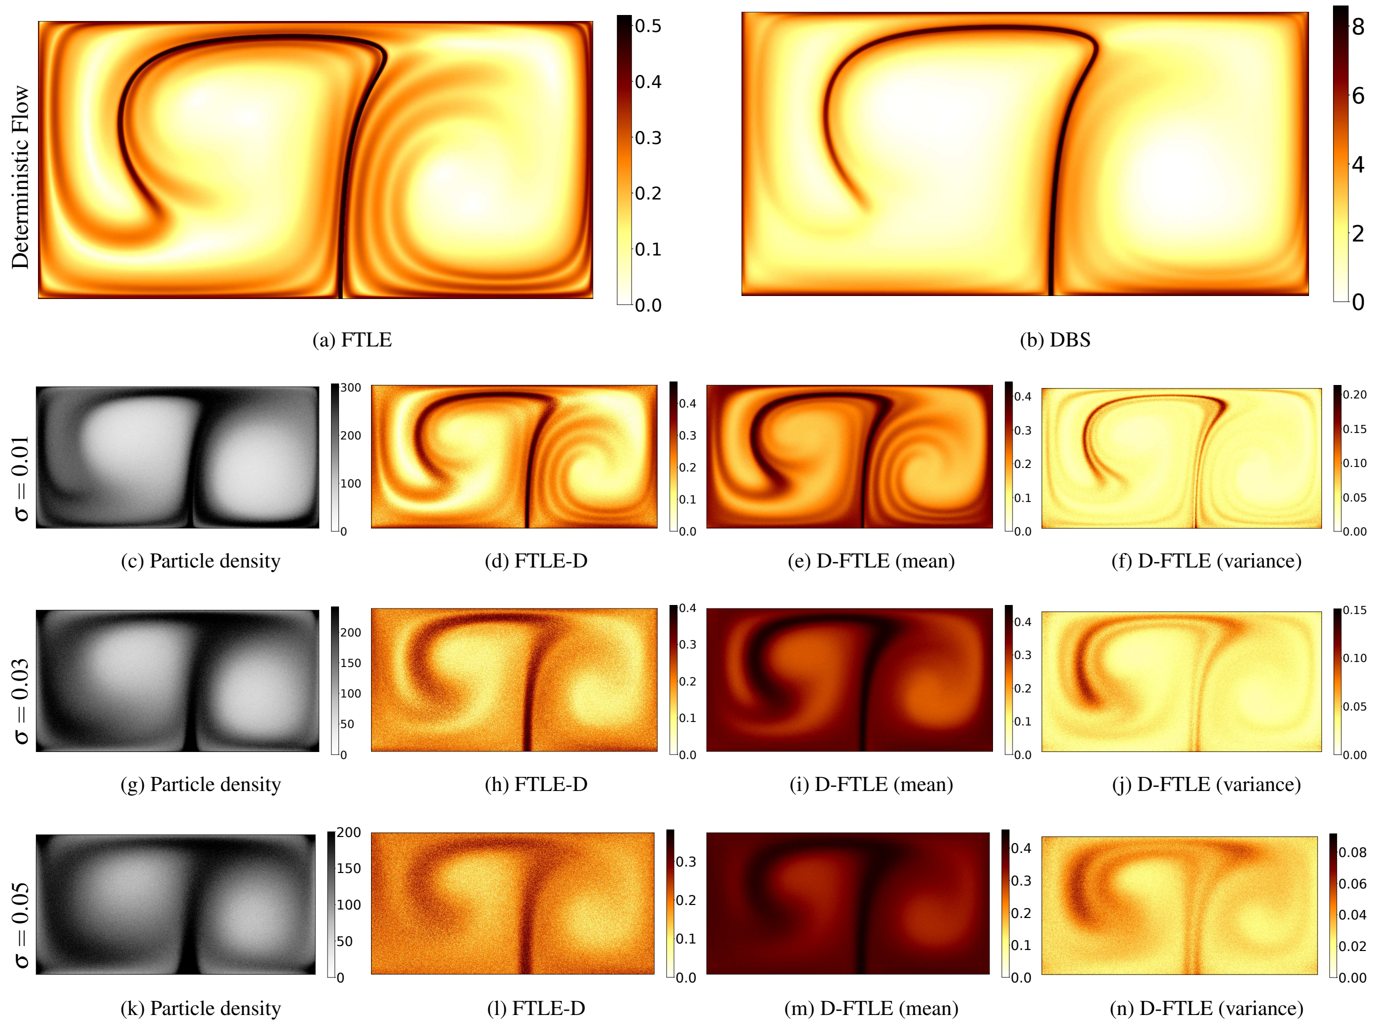


(a) FTLE (b) DBS

(c) Particle density (d) FTLE-D (e) D-FTLE (mean) (f) D-FTLE (variance)

(g) Particle density (h) FTLE-D (i) D-FTLE (mean) (j) D-FTLE (variance)

(k) Particle density (l) FTLE-D (m) D-FTLE (mean) (n) D-FTLE (variance)

Figure 1: The double gyre dataset with different amounts of isotropic Gaussian noise. In (a) and (b) the FTLE and DBS of the deterministic flow are shown. Note that the DBS is not affected by changing the amount of isotropic noise.

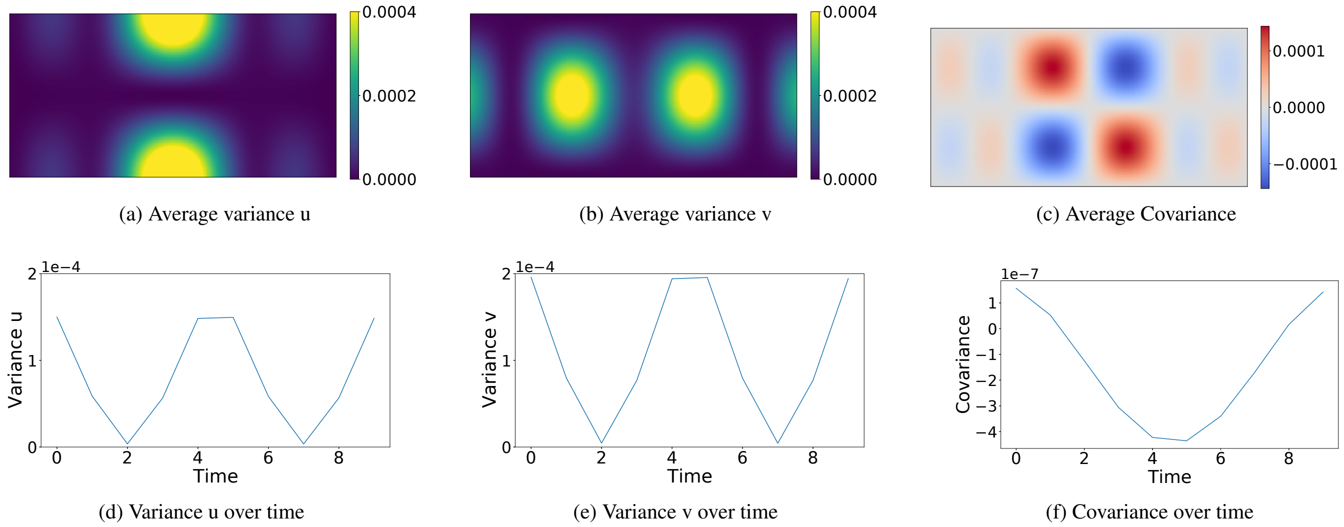


(a) Average variance u (b) Average variance v (c) Average Covariance

(d) Variance u over time (e) Variance v over time (f) Covariance over time

Figure 2: Gaussian error model of the double gyre reduced to a resolution of $[256 \times 128 \times 10]$.

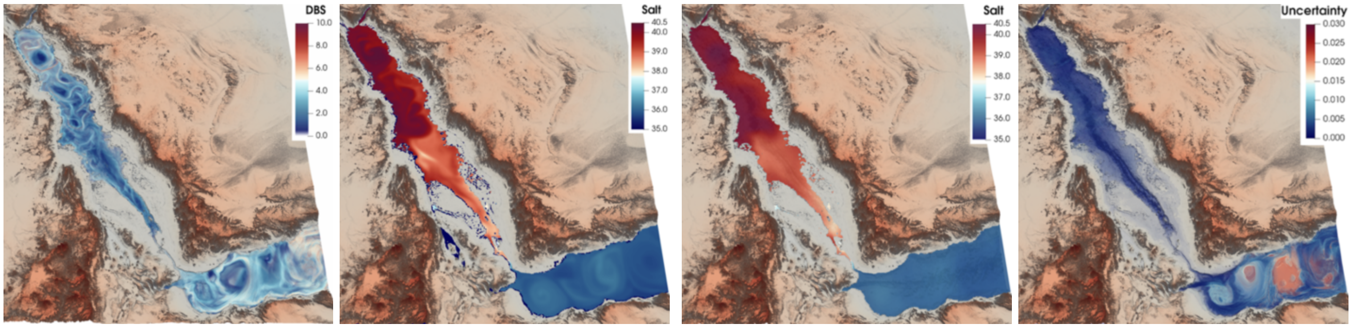


(a) Forward DBS (b) Salinity $t_0$ (c) Salinity $t_1$ (d) Transport uncertainty

Figure 3: The forward DBS in (a) visualizes transport barriers in the uncertain flow. The salinity concentration at time $t_0$ and $t_1$ is shown in (b) and (c).

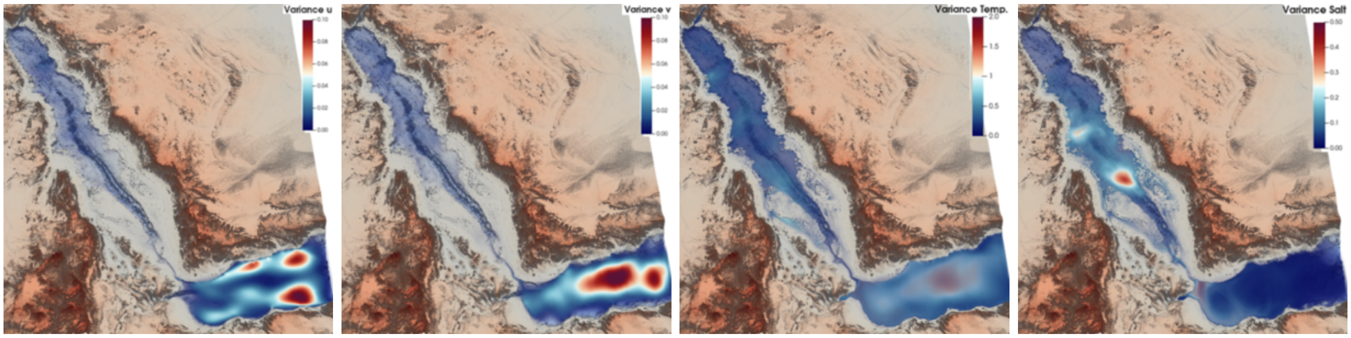


(a) Variance $u$ (b) Variance $v$ (c) Variance of temperature (d) Variance of salinity

Figure 4: Volume rendering of the time-averaged variance in the Red Sea dataset estimated from the ensemble members. Variance in $w$-direction, i.e. along the depth axis, is not shown here since it is close to zero.

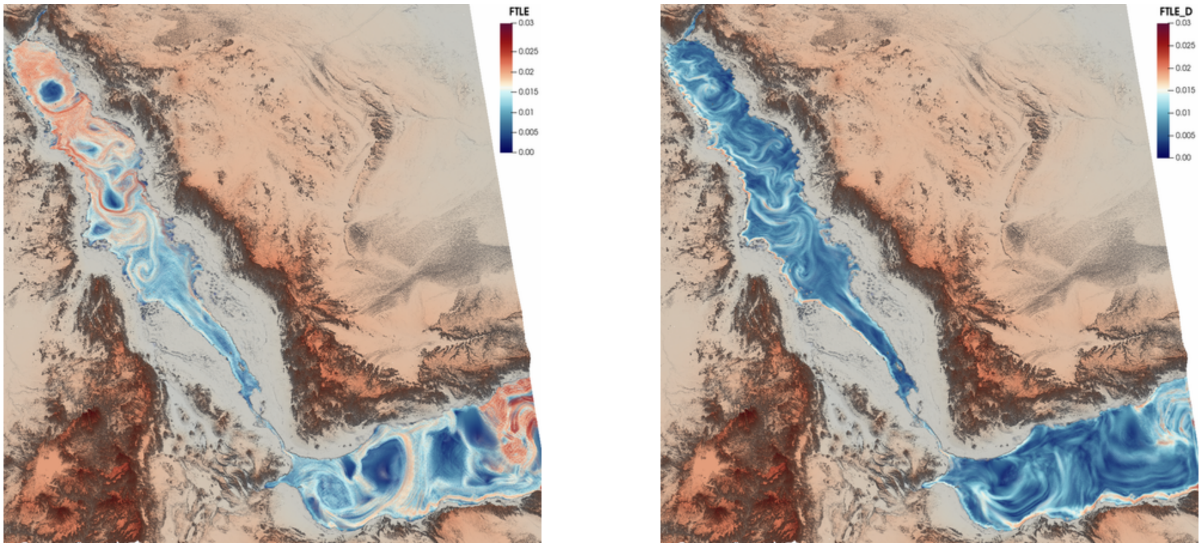


(a) Forward FTLE (b) Forward FTLE-D

Figure 5: The forward FTLE of the mean flow is shown in (a) and the forward FTLE-D of the stochastic flow is visualized in (b).

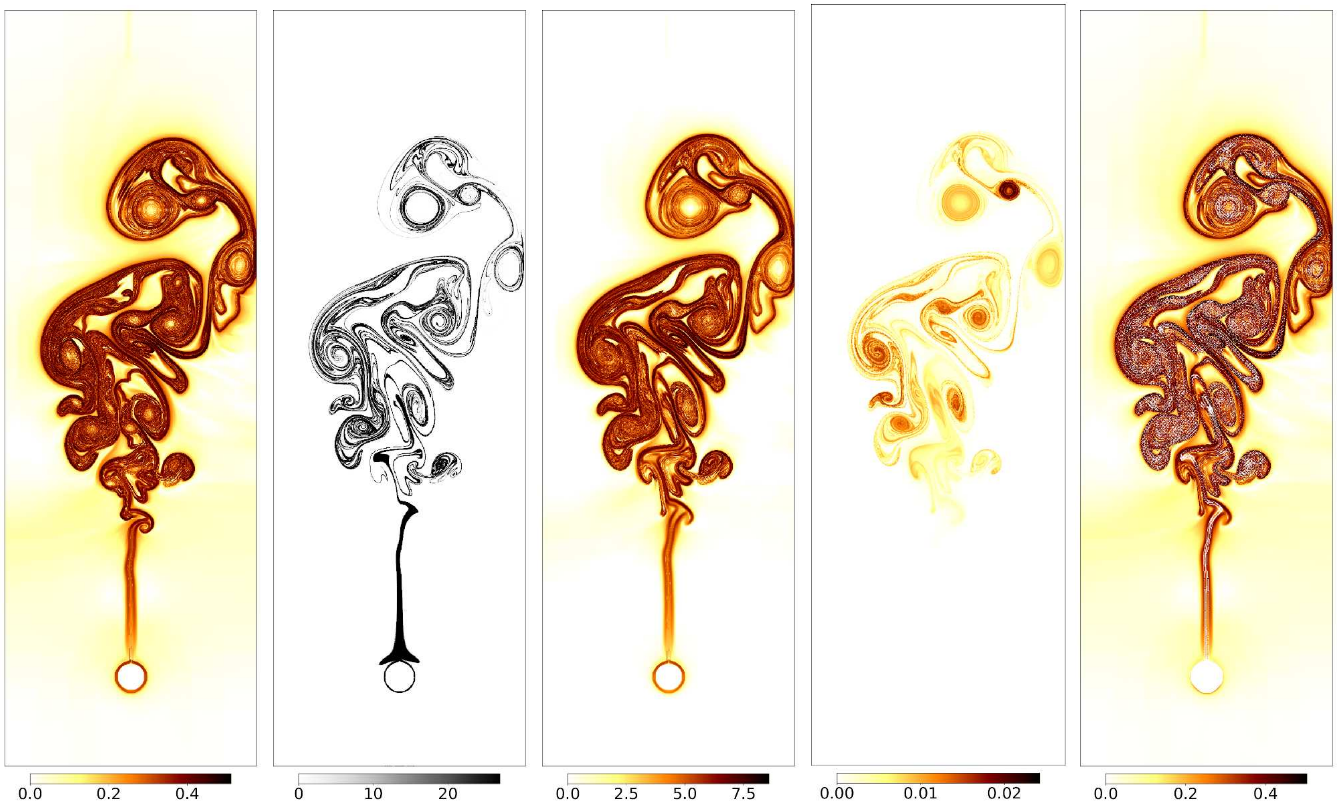


(a) Deterministic FTLE (b) Particle density (c) DBS (d) Transport uncertainty (e) FTLE-D

Figure 6: The heated cylinder dataset with uncertainty estimated during data reduction to a grid of size $[150 \times 450 \times 100]$.

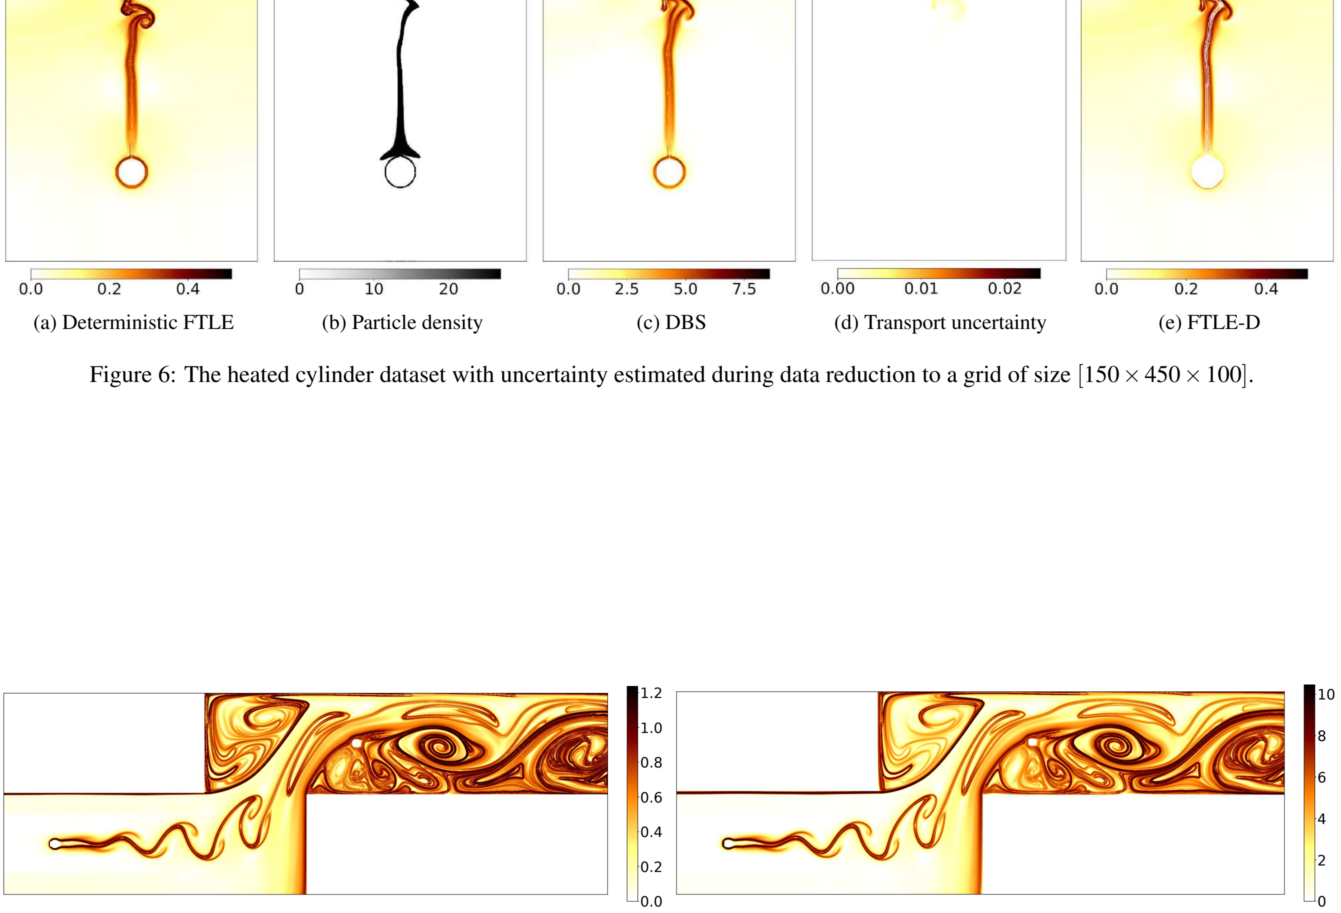


(a) FTLE (b) DBS

Figure 7: The backward FTLE (a) and DBS (b) of the deterministic flow around corners.
